# Supplementary material for: HumanEval Pro and MBPP Pro: Evaluating Large Language Models on Self-invoking Code Generation
Source: arXiv:2412.21199 source file (2024-12-31)
Supplement: Supplementary file 1 [file appendix-error-examples.tex]

\section{Examples in Correctness Verification}
\label{app:error}
\begin{lstlisting}[caption=SyntaxError in HumanEval/47, basicstyle=\ttfamily]
Status: Failed
Error:  File "./humanevalpro/case_47/gen_0.py", line 29
    fib4(0) -> 0
            ^^
SyntaxError: invalid syntax
\end{lstlisting}
\begin{lstlisting}[basicstyle=\ttfamily]
def fib4(n: int):
    """The Fib4 number sequence is a sequence similar to the Fibbonacci sequnece that's defined as follows:
    fib4(0) -> 0
    fib4(1) -> 0
    fib4(2) -> 2
    fib4(3) -> 0
    fib4(n) -> fib4(n-1) + fib4(n-2) + fib4(n-3) + fib4(n-4).
    Please write a function to efficiently compute the n-th element of the fib4 number sequence.  Do not use recursion.
    >>> fib4(5)
    4
    >>> fib4(6)
    8
    >>> fib4(7)
    14
    """

    results = [0, 0, 2, 0]
    if n < 4:
        return results[n]

    for _ in range(4, n + 1):
        results.append(results[-1] + results[-2] + results[-3] + results[-4])
        results.pop(0)

    return results[-1]

# Given a list of integers, compute the sum of the Fib4 values for each integer in the list. If the list contains duplicate integers, compute the Fib4 value only once for each unique integer and then sum these values. Return the total sum as the result.
# The Fib4 number sequence is a sequence similar to the Fibonacci sequence that's defined as follows:
|{\colorbox{lightred}{fib4(0) -> 0}}|
|{\colorbox{lightred}{fib4(1) -> 0}}|
|{\colorbox{lightred}{fib4(2) -> 2}}|
|{\colorbox{lightred}{fib4(3) -> 0}}|
|{\colorbox{lightred}{fib4(n) -> fib4(n-1) + fib4(n-2) + fib4(n-3) + fib4(n-4)}}|

|{\colorbox{lightblue}{Fixed: }}|
|{\colorbox{lightblue}{"""}}|
|{\colorbox{lightblue}{fib4(0) -> 0}}|
|{\colorbox{lightblue}{fib4(1) -> 0}}|
|{\colorbox{lightblue}{fib4(2) -> 2}}|
|{\colorbox{lightblue}{fib4(3) -> 0}}|
|{\colorbox{lightblue}{fib4(n) -> fib4(n-1) + fib4(n-2) + fib4(n-3) + fib4(n-4)}}|
|{\colorbox{lightblue}{"""}}|

from typing import List
def sum_fib4_values(lst: List[int]) -> int:
    unique_numbers = set(lst)
    total_sum = sum(fib4(n) for n in unique_numbers)
    return total_sum

assert sum_fib4_values([5, 6, 7]) == 26
assert sum_fib4_values([0, 1, 2, 3]) == 2
assert sum_fib4_values([5, 5, 6, 6, 7, 7]) == 26
assert sum_fib4_values([10, 11, 12]) == 690
assert sum_fib4_values([]) == 0
\end{lstlisting}

\begin{lstlisting}[caption=SyntaxError in HumanEval/47, basicstyle=\ttfamily]
Status: Failed
Error:Traceback (most recent call last):
  File "/work/zhuotaodeng/yzj/evalpro/mbpppro/v0.2/log/case_216/gen_0.py", line 17, in <module>
    assert SumOfFirstElements([[10], [20, 30], [], [40, 50, 60]]) == 70
  File "/work/zhuotaodeng/yzj/evalpro/mbpppro/v0.2/log/case_216/gen_0.py", line 10, in SumOfFirstElements
    extracted_elements = Extract(lst)
  File "/work/zhuotaodeng/yzj/evalpro/mbpppro/v0.2/log/case_216/gen_0.py", line 5, in Extract
    return [item[0] for item in lst] 
  File "/work/zhuotaodeng/yzj/evalpro/mbpppro/v0.2/log/case_216/gen_0.py", line 5, in <listcomp>
    return [item[0] for item in lst] 
IndexError: list index out of range
\end{lstlisting}
\begin{lstlisting}[basicstyle=\ttfamily]
# Write a python function to get the first element of each sublist.

def Extract(lst): 
    return [item[0] for item in lst] 


# Given a list of lists, where each sublist contains multiple elements, write a function to extract the first element of each sublist and then find the sum of these extracted elements. If a sublist is empty, it should be ignored in the sum calculation.
def SumOfFirstElements(lst):
    extracted_elements = Extract(lst)
    return sum(element for element in extracted_elements if element is not None)

assert SumOfFirstElements([[1, 2], [3, 4], [5, 6]]) == 9
assert SumOfFirstElements([[10], [20, 30], [], [40, 50, 60]]) == 70
assert SumOfFirstElements([[], [1], [2, 3], [4, 5, 6]]) == 7
assert SumOfFirstElements([[0], [0], [0]]) == 0
assert SumOfFirstElements([[1, 2, 3], [], [4, 5], [6]]) == 11
\end{lstlisting}
